# Supplementary material for: A study guide for the $\ell^2$ decoupling theorem for the paraboloid
Source: arXiv:2402.14756 source file (2024-02-22)
Supplement: Supplementary file 1 [file appendix_applications_to_number_theory.tex]

One of the highlights of the decoupling theory is the resolution of Vinogradov's main conjecture. It is surprising that the proof solely relies on decoupling theory for the moment curve and doesn't resort to any deep number theory. Now we only briefly introduce the problem (for more historical remarks see \cite{pierce2017vinogradov}). Fix any positive integers $k,s$, consider the Vinogradov's system of equations of degree $k$:
\begin{align*}
    x_1+x_2+...+x_s&=y_1+y_2+...+y_s\\
    x_1^2+x_2^2+...+x_s^2&=y_1^2+y_2^2+...+y_s^2\\
    x_1^3+x_2^3+...+x_s^3&=y_1^3+y_2^3+...+y_s^3\\
    &\vdots\\
    x_1^k+x_2^k+...+x_s^k&=y_1^k+y_2^k+...+y_s^k.
\end{align*}

Let $J_{s,k}(X)$ be the number of the integer solutions to the system of equations above with $1\leq x_i,y_i\leq X$ for all $1\leq i \leq s$. Vinogradov's main conjecture predicts that for all $\epsilon>0$, we have
\begin{align*}
    J_{s,k}(X) \lesssim_\e X^{s+\epsilon}+X^{2s-\frac{1}{2}k(k+1)+\epsilon}.
\end{align*}

The term $X^{s+\epsilon}$ corresponds to diagonal solutions, i.e., the solutions with $x_i=y_i$ for all $1\leq i \leq s$. The term $X^{2s-\frac{1}{2}k(k+1)+\epsilon}$ corresponds to generic solutions, and the order $2s-\frac{1}{2}k(k+1)$ could be predicted by random heuristics. In fact, we have matching lower bound:
\begin{align*}
    X^{s}+X^{2s-\frac{1}{2}k(k+1)}\lesssim J_{s,k}(X)
\end{align*}

Hence, Vinogradov's main conjecture is sharp up to $\epsilon$ loss. (Coincidentally, decoupling estimates also have epsilon loss.) Vinogradov's main conjectures were proved independently first by Bourgain, Demeter and Guth \cite{bourgain_proof_2016}\footnote{which also points out that $X^\e$ loss can be removed for $s>\frac{1}{2}k(k+1)$.} via the sharp $\ell^2$ decoupling inequality for the moment curve, and later by Wooley m\cite{wooley_nested_2019} via nested efficient congruencing argument. It turns out that these two seemingly irrelevant approaches have some deep connections, for which \cite{pierce2017vinogradov} is an excellent resource. One noteworthy achievement towards this direction is \cite{guo2021short}, which borrows insights from \cite{wooley_nested_2019} to give a short alternative proof of the $\ell^2$ decoupling inequality for the moment curve.

It is natural to wonder why it is important to investigate Vinogradov's system. Here are some motivations.

Let's first recall Waring's problem. We know that every positive integer is a sum of $4$ squares, a sum of $9$ cubes and a sum of $19$ fourth powers. Now given any positive integer $k$, is every positive integer a sum of finitely many $k$-th powers? If so, what is the least number of the $k$-th powers we need? Classically, we have

\begin{align*}
    \#\{(x_1,x_2,...,x_s)\in \mathbb{N}^s:n=x_1^k+x_2^k+...+x_s^k\}\approx \Gamma\left(1+\frac{1}{k}\right)^s \Gamma\left(\frac{s}{k}\right)^{-1} n^{\frac{s}{k}-1}
\end{align*}

\noindent when $s>2^k$. With the help of  Vinogradov's main conjecture, this bound can be improved to $s\gg k^2$.

Another motivation is the zero-free region of the Riemann zeta function. With innumerous implications, the distribution of the zeroes of the Riemann zeta function $\zeta(s)$ has long been a central topic in number theory. For example, the prime number theorem is equivalent to the fact that there is no zero on the line $\on{Re}(s)=1$. The Riemann hypothesis conjectures that all non-trivial zeroes are on the critical line $\on{Re}(s)=\frac{1}{2}$. The classical zero-free region is

$$\{\sigma+it: \sigma>1-\frac{c}{\log(|t|+2)}\}$$

\noindent with some absolute constant $c$. And Vinogradov's system is closely related to extending the zero-free region to 

$$\{\sigma+it: \sigma>1-\frac{c^{\prime}}{\log(|t|+100)^{\frac{2}{3}}(\log\log(|t|+100))^{\frac{1}{3}}}\}$$

\noindent with some absolute constant $c^{\prime}$.
